# Supplementary material for: Network Fault-tolerant and Byzantine-resilient Social Learning via Collaborative Hierarchical Non-Bayesian Learning
Source: arXiv:2307.14952 source file (2023-07-27)
Supplement: Supplementary file 1 [file appendix.tex]

\section{State Estimation Proofs}

\begin{proof}
When $\sum_{j=1}^n\pth{H_j^{\top}H_j}$ is invertible, $f_i$ has a unique minimizer $w_i^{*}$. 

By definition of the global objective of a single network $f_i$, we have 
 \begin{IEEEeqnarray}{c}
f\pth{\hat{w}_j^{i}[T]} - f(w_i^{*})  = \pth{w_j^{i}-w_i^{*}}^{\top}\sum_{j=1}^n\pth{H_j^{\top}H_j}\pth{w_j^{i}-w_i^{*}} 
 \\ \ge\lambda_{\min}\pth{\sum_{j=1}^n\pth{H_j^{\top}H_j}}\norm{w_j^{i}-w_i^{*}}^2.
 \end{IEEEeqnarray}

Fix a time horizon $T$. Since $w_i^{*}\in \calW$, we have 
 \begin{multline}
\lambda_{\min}\pth{\sum_{j=1}^{n_i}\pth{H_j^{\top}H_j}}\norm{w-w_i^{*}}^2 
 \le f\pth{\hat{w}_j^{i}[T]} - f(w_i^{*}) \\
  = f\pth{\hat{v}[T]} - f(w_i^{*}) + f\pth{\hat{w}_j^{i}[T]} - f\pth{v[T]} \\
  \le f\pth{\hat{v}[T]} - f(w_i^{*}) + L\norm{\hat{w}_j^{i}[T] - \hat{v}[T]}, ~~~ \text{by Proposition \ref{prop: lipschitz}} \\
  = f\pth{\frac{1}{T}\sum_{t=1}^T v[t]} - f(w_i^{*}) + L\norm{\frac{1}{T}\sum_{t=1}^Tw_j^{i}[t] - \frac{1}{T}\sum_{t=1}^Tv[t]} \\
  \le \frac{1}{T}\sum_{t=1}^T f(v[t]) - f(w_i^{*}) + \frac{1}{T}\sum_{t=1}^T L \norm{w_j^{i}[t] - v[t]} \\
  \le  \frac{1}{T}\sum_{t=1}^T f(v[t]) - f(w_i^{*}) + \frac{1}{T}\sum_{t=1}^T L \alpha[t-1]\norm{\bar{z}^{i}[t] -\frac{z_j^{i}[t]}{m_j^{i}[t]}}. 
 \end{multline}
For the first term, we have 
 \begin{multline}
\frac{1}{T}\sum_{t=1}^T f(v[t]) - f(w_i^{*})   =  \frac{1}{T}\sum_{t=1}^T \sum_{i=1}^n f_i(w_i[t]) - f(w_i^{*})
\\+ \frac{1}{T}\sum_{t=1}^T f(v[t]) - \frac{1}{T}\sum_{t=1}^T \sum_{i=1}^n f_i(w_i[t]) \\
  = \frac{1}{T}\sum_{t=1}^T \sum_{i=1}^n f_i(w_i[t]) - \sum_{i=1}^n f_i(w_i^{*}) 
+ \frac{1}{T}\sum_{t=1}^T \sum_{i=1}^n f_i((v[t]) - \\\frac{1}{T}\sum_{t=1}^T \sum_{i=1}^n f_i(w_i[t])\\
  \le \frac{1}{T}\sum_{t=1}^T \sum_{i=1}^n f_i(w_i[t]) - \sum_{i=1}^n f_i(w_i^{*}) 
+ \\\frac{1}{T}\sum_{t=1}^T \sum_{i=1}^n L\norm{v[t] -w_i[t]}, ~~~ \text{by Proposition \ref{prop: lipschitz}}\\
  \le \frac{1}{T}\sum_{t=1}^T \sum_{i=1}^n f_i(w_i[t]) - \sum_{i=1}^n f_i(w_i^{*}) 
+ \\\frac{1}{T}\sum_{t=1}^T \sum_{i=1}^n L\alpha[t-1]\norm{\bar{z}[t] -\frac{z_i[t]}{m_i[t]}}
\end{multline}

Since $f_i$ is convex for each $i=1, \cdots, n$, it holds that 
 \begin{IEEEeqnarray}{c}
f_i(w_i[t]) - f_i(w_i^{*})  \le \iprod{\nabla f_i(w_i[t])}{w_i[t] - w} \\
  = \iprod{g_i^{\prime}[t]}{w_i[t] - w} \\
  = \iprod{g_i[t]}{w_i[t] - w} + \iprod{g_i^{\prime}[t] - g_i[t]}{w_i[t] - w} 
 \end{IEEEeqnarray}

We have 
\begin{multline}
\frac{1}{T}\sum_{t=1}^T \sum_{i=1}^n f_i(w_i[t]) - \sum_{i=1}^n f_i(w^*) 
 \\\le  \frac{1}{T}\sum_{t=1}^T \sum_{i=1}^n \iprod{g_i[t]}{w_i[t] - w} + \iprod{g_i^{\prime}[t] - g_i[t]}{w_i[t] - w}
 \\ = \frac{1}{T}\sum_{i=1}^n \sum_{t=1}^T \iprod{g_i[t]}{w_i[t] - w} + \\\frac{1}{T}\sum_{i=1}^n \sum_{t=1}^T \iprod{g_i^{\prime}[t] - g_i[t]}{w_i[t] - w}
 \\ \le \frac{1}{2T}\sum_{i=1}^n\sum_{t=1}^T \alpha[t-1] \norm{g_i[t]}^2 + \frac{n}{T\alpha[T]}\varphi(w) + \\ \frac{1}{T}\sum_{i=1}^n \sum_{t=1}^T \iprod{g_i^{\prime}[t] - g_i[t]}{w_i[t] - w}. 
\end{multline}

\paragraph{Bounding $\norm{\bar{z}^{i}[t]-\frac{z_j^{i}[t]}{m_j^{i}[t]}}$:}

\begin{multline}
\norm{\bar{z}^{i}[t]-\frac{z_j^{i}[t]}{m_j^{i}[t]}} 
 = \\
\norm{\frac{1}{n_i} \sum_{r=0}^{t-1}\sum_{j^{\prime}=1}^{n_i} g_{j^{\prime}}^{i}[r] -\frac{\sum_{r=0}^{t-1}\sum_{j^{\prime}=1}^{n_i} g_{j^{\prime}}^{i}[r] {\bf \Psi}_{j^{\prime},j}(r,t)}{\sum_{j^{\prime}=1}^{n_i}{\bf \Psi}_{j^{\prime},j}(1,t)} }\\
 \\ = \norm{\frac{\sum_{r=0}^{t-1} \sum_{j^{\prime}=1}^{n_i} g_{j^{\prime}}^{i}[r] \sum_{k=1}^{n_i} \pth{ {\bf \Psi}_{k,j}(1, t) -  {\bf \Psi}_{j^{\prime},j}(r, t)}   }{{n_i} \sum_{j^{\prime}=1}^{{n_i}}{\bf \Psi}_{j^{\prime},j}(1,t)} }\\
 \le \frac{\norm{\sum_{r=0}^{t-1} \sum_{j^{\prime}=1}^{n_i} g_{j^{\prime}}^{i}[r] \sum_{k=1}^{n_i} \pth{ {\bf \Psi}_{k,j}(1, t) -  {\bf \Psi}_{j^{\prime},j}(r, t)}  } }{ {n_i} {n_i}  \beta^{{n_i}B+1}} \\
 \le \frac{ L \sum_{r=0}^{t-1} \sum_{j^{\prime}=1}^{n_i} \sum_{k=1}^{n_i} \norm{ {\bf \Psi}_{k,j}(1, t) -  {\bf \Psi}_{j^{\prime},j}(r, t)}}{{n_i}^2  \beta^{{n_i}B+1}}
\end{multline}
We know that 
\begin{multline}
\norm{ {\bf \Psi}_{k,j}(1, t) -  {\bf \Psi}_{j^{\prime},j}(r, t)} \\  = \norm{\sum_{p=1}^m {\bf \Psi}_{k,p}(1, r-1) {\bf \Psi}_{p,j}(r, t) -  {\bf \Psi}_{j^{\prime},j}(r, t)}\\
% = \norm{\sum_{p=1}^m {\bf \Psi}_{k,p}(1, r-1) \pth{{\bf \Psi}_{p,i}(r, t) -  {\bf \Psi}_{j,i}(r, t)}}\\
 \le \sum_{p=1}^m {\bf \Psi}_{k,p}(1, r-1) \norm{{\bf \Psi}_{p,j}(r, t) -  {\bf \Psi}_{j^{\prime},j}(r, t)}
 \le \gamma^{\lfloor \frac{t-r+1}{{n_i}B+1}\rfloor}. 
\end{multline}
Thus, we have 
 \begin{equation}
\norm{\bar{z}^{i}[t]-\frac{z_j^{i}[t]}{w_j^{i}[t]}} \le \frac{L}{\beta^{{n_i}B+1}(1-\gamma^{\frac{1}{{n_i}B+1}})  \gamma^{\frac{{n_i}B}{{n_i}B+1}}}.
 \end{equation}

\end{proof}

\paragraph{Bounding $\frac{1}{T}\sum_{i=1}^n \sum_{t=1}^T \iprod{g_i^{\prime}[t] - g_i[t]}{w_i[t] - w^*}$.}

It can be easily checked by definition that $\iprod{g_i^{\prime}[t] - g_i[t]}{w_i[t] - w^*}$ is a martingale. 
By the Cauchy–Schwartz inequality, we have  
\begin{multline}
\abth{\iprod{g_i^{\prime}[t] - g_i[t]}{w_i[t] - w^*}} \\ \le \norm{g_i^{\prime}[t] - g_i[t]}\norm{w_i[t] - w^*} \le 2LR.     
\end{multline}
That is, $\iprod{g_i^{\prime}[t] - g_i[t]}{w_i[t] - w^*}$ is a bounded difference martingale. By Azuma's inequality, with probability at least $1-\delta$, it holds that 
 \begin{equation}
\frac{1}{nT}\sum_{t=1}^T \sum_{i=1}^n \iprod{g_i^{\prime}[t] - g_i[t]}{w_i[t] - w^*} \le 4LR\sqrt{\frac{\log \frac{1}{\delta}}{T}}.     
 \end{equation}

 \section{Tracking Proofs}
 \begin{proof}[Proof of Theorem \ref{thm: convergence of hierarchical FL: tracking}]
The local estimate at each agent $j$ is $w_j[t] = \frac{z_j[t]}{m_j[t]}$. 
We first observe that the evolution of $\bar{z}$  can be formally described as 
\begin{align*}
\bar{z}[t+1] & = \frac{1}{N}\sum_{j=1}^{\tilde{N}}z_j[t+1]  
= -\frac{1}{N}\sum_{r=1}^{t+1}  A^{t+1-r} \eta[r]\sum_{j^{\prime}=1}^{N}g_{j^{\prime}}[r] \\
& = -\frac{1}{N} \pth{A \sum_{r=1}^{t}  A^{t-r} \eta[r]\sum_{j^{\prime}=1}^{N}g_{j^{\prime}}[r] + \eta[t+1]\sum_{j^{\prime}=1}^{N}g_{j^{\prime}}[t+1]}  \\
& = A \bar{z}[t] - \eta[t+1]\frac{1}{N}\sum_{j^{\prime}=1}^{N}g_{j^{\prime}}[t+1]. 
\end{align*}
We bound the amortized tracking error at any arbitrary agent $j$ as follows: 
\begin{align}
\label{eq: tracking average cumultive error}
\frac{1}{T}\sum_{t=1}^T \pth{w_j[t] - w_t^*} 
& =  \underbrace{\frac{1}{T}\sum_{t=1}^T \pth{\bar{z}[t] - w_t^*}}_{(a)} + \underbrace{\frac{1}{T}\sum_{t=1}^T \pth{w_j[t] - \bar{z}[t]}}_{(b)}. 
% \frac{1}{T}\sum_{t=1}^T \sum_{j=1}^{N} f_j(w_j[t]) - f(w_t^{*})
% + \frac{1}{T}\sum_{t=1}^T f(v[t]) - \frac{1}{T}\sum_{t=1}^T \sum_{j=1}^{N} f_j(w_j[t]) \\
% & = \frac{1}{T}\sum_{t=1}^T \sum_{j=1}^{N} f_j(w_j[t]) - \sum_{j=1}^{N} f_j(w_t^{*}) 
% + \frac{1}{T}\sum_{t=1}^T \sum_{j=1}^{N} f_j((v[t]) - \frac{1}{T}\sum_{t=1}^T \sum_{j=1}^{N} f_j(w_j[t])\\
% & \le \frac{1}{T}\sum_{t=1}^T \sum_{j=1}^{N} f_j(w_j[t]) - \sum_{j=1}^{N} f_j(w_t^{*}) 
% + \frac{1}{T}\sum_{t=1}^T \sum_{j=1}^{N} L\norm{v[t] -w_j[t]}, ~~~ \text{by Proposition \ref{prop: lipschitz}}\\
% & \le \frac{1}{T}\sum_{t=1}^T \sum_{j=1}^{N} f_j(w_j[t]) - \sum_{j=1}^{N} f_j(w_t^{*}) 
% + \frac{1}{T}\sum_{t=1}^T \sum_{j=1}^{N} L\alpha[t-1]\norm{\bar{z}[t] -\frac{z_j[t]}{m_j[t]}}
\end{align}

\paragraph{Bounding (b):}
\begin{align*}
\norm{w_j[t] - \bar{z}[t]}  &=  \norm{\frac{w_j[t]}{m_j[t]} - \bar{z}[t]} 
 = \norm{\frac{\sum_{r=0}^{t-1}\sum_{j^{\prime}=1}^{N} A^{t-r}\eta[r]g_{j^{\prime}}^{i}[r] {\bf \Psi}_{j^{\prime},j}(r,t)}{\sum_{j^{\prime}=1}^{N}{\bf \Psi}_{j^{\prime},j}(1,t)} - \frac{1}{N}\sum_{r=1}^{t}  A^{t-r}\eta[r]\sum_{j^{\prime}=1}^{N}g_{j^{\prime}}[r]} \\
 & = \norm{\frac{\sum_{r=0}^{t-1} \sum_{j^{\prime}=1}^{N} A^{t-r}\eta[r]g_{j^{\prime}}^{i}[r] \sum_{k=1}^{N} \pth{ {\bf \Psi}_{k,j}(1, t) -  {\bf \Psi}_{j^{\prime},j}(r, t)}   }{{N} \sum_{j^{\prime}=1}^{{N}}{\bf \Psi}_{j^{\prime},j}(1,t)} }\\
 & \le \frac{4M^2\norm{\sum_{r=0}^{t-1} \sum_{j^{\prime}=1}^{N} A^{t-r}\eta[r] g_{j^{\prime}}^{i}[r] \sum_{k=1}^{N} \pth{ {\bf \Psi}_{k,j}(1, t) -  {\bf \Psi}_{j^{\prime},j}(r, t)}  } }{ N^2  \pth{\min_{i\in [M]}\beta_i}^{2D^*B}} \\
 & \overset{(a)}{\le} \frac{4M^2L\sum_{r=0}^{t-1} \sum_{j^{\prime}=1}^{N} \norm{A}^{t-r}\eta[r]  \abth{\sum_{k=1}^{N} \pth{ {\bf \Psi}_{k,j}(1, t) -  {\bf \Psi}_{j^{\prime},j}(r, t)}  } }{ N^2  \pth{\min_{i\in [M]}\beta_i}^{2D^*B}} \\
 & =  \frac{4M^2L\sum_{r=0}^{t-1} \sum_{j^{\prime}=1}^{N} \norm{A}^{t-r}\eta[r]  \abth{\sum_{k=1}^{N} \pth{ \sum_{p=1}^N{\bf \Psi}_{k,p}(1, r-1){\bf \Psi}_{p,j}(r, t) -  {\bf \Psi}_{j^{\prime},j}(r, t)}}}{ N^2  \pth{\min_{i\in [M]}\beta_i}^{2D^*B}}
\\
& \le \frac{4M^2L\sum_{r=0}^{t-1} \sum_{j^{\prime}=1}^{N} \norm{A}^{t-r}\eta[r]  \sum_{k=1}^{N} \sum_{p=1}^N{\bf \Psi}_{k,p}(1, r-1)\abth{{\bf \Psi}_{p,j}(r, t) -  {\bf \Psi}_{j^{\prime},j}(r, t)}}{ N^2  \pth{\min_{i\in [M]}\beta_i}^{2D^*B}} \\
& \le \frac{4M^2L\sum_{r=0}^{t-1} \sum_{j^{\prime}=1}^{N} \norm{A}^{t-r}\eta[r] \delta\pth{{\bf \Psi}(r,t)}}{ N  \pth{\min_{i\in [M]}\beta_i}^{2D^*B}} \\
& \overset{(b)}{\le} \frac{4M^2L\sum_{r=0}^{t-1}  \norm{A}^{t-r}\eta[r] \gamma^{\frac{t-r}{\Gamma}}}{\pth{\min_{i\in [M]}\beta_i}^{2D^*B}}\\
& = \frac{4M^2L\sum_{r=0}^{t-1} \eta[r] \pth{\norm{A}\gamma^{\frac{1}{\Gamma}}}^{t-r}}{\pth{\min_{i\in [M]}\beta_i}^{2D^*B}}, 
\end{align*}
where the inequality (a) holds because of Claim \ref{claim: bounded stochastic gradient} and 
the inequality (b) follows from Lemma \ref{lm: matrix block rate}.

For ease of exposition, let $b= \norm{A}\gamma^{\frac{1}{\Gamma}}$. Let $r^*\in \{1, 2, \cdots, t-1\}$. 
It holds that 
\begin{align*}
\sum_{r=0}^{t-1} \eta[r] \pth{\norm{A}\gamma^{\frac{1}{\Gamma}}}^{t-r}   
& = \sum_{r=0}^{t-1} \eta[r] b^{t-r} \\
& = \frac{1}{\norm{K}}\pth{\sum_{r=1}^{t-1} \frac{1}{r} b^{t-r} + b^t} \\ 
& = \frac{1}{\norm{K}}\pth{\underbrace{b^t + \sum_{r=1}^{r^*} \frac{1}{r} b^{t-r}}_{(i)} + \underbrace{\sum_{r=r^* + 1}^{t-1} \frac{1}{r} b^{t-r}}_{(ii)}}. 
\end{align*}
Term (i) can be upper bounded as 
\begin{align*}
b^t + \sum_{r=1}^{r^*} \frac{1}{r} b^{t-r}  \le b^t + \sum_{r=1}^{r^*} b^{t-r} = \sum_{r=0}^{r^*} b^{t-r} \le \frac{b^{t-r^*}}{1-b}, \qquad \qquad \qquad \qquad \qquad \qquad \qquad \hfill \text{(ub\,$(i)$)} 
\end{align*}
and term (ii) can be upper bounded as 
\begin{align*}
\sum_{r=r^* + 1}^{t-1} \frac{1}{r} b^{t-r} 
\le \sum_{r=r^* + 1}^{t-1} \frac{1}{r^*+1} b^{t-r} 
= \frac{1}{r^*+1} \sum_{r=r^* + 1}^{t-1} b^{t-r} 
\le \frac{1}{(r^*+1)(1-b)}. \qquad \qquad  \text{(ub\,$(ii)$)}   
\end{align*}
Choosing $r^* = 1/2 t$, when 
\begin{align}
\label{eq: threshold time}
t \ge \frac{2}{\log 1/b} \log \pth{\frac{2}{\log 1/b}}  ~ \triangleq ~ t_0, 
\end{align}
where the base of the log is $2$, both of the upper bounds above can be further upper bounded as $\frac{2}{(1-b)t}$. Thus, 
\begin{align*}
\sum_{r=0}^{t-1} \eta[r] \pth{\norm{A}\gamma^{\frac{1}{\Gamma}}}^{t-r} \le \frac{4}{(1-b)t}~~~ \qquad \forall t\ge t_0. 
\end{align*}
For $t<t_0$, it holds that 
\begin{align*}
\sum_{r=0}^{t-1} \eta[r] \pth{\norm{A}\gamma^{\frac{1}{\Gamma}}}^{t-r} 
\le \sum_{r=0}^{t-1} \eta[r] 
\le \sum_{r=0}^{t-1}
\le \sum_{r=0}^{t_0-1}
=t_0. 
\end{align*}
Therefore, 
\begin{align*}
\norm{w_j[t] - \bar{z}[t]} 
\le 
\begin{cases}
\frac{16M^2L}{\pth{\min_{i\in [M]}\beta_i}^{2D^*B}\norm{K}(1-b)t}, ~~~ ~~ &\text{if } ~ t \ge t_0; \\ 
\frac{4M^2Lt_0}{\pth{\min_{i\in [M]}\beta_i}^{2D^*B}\norm{K}}, ~~~ ~~ &\text{if } ~ t < t_0, 
\end{cases}
\end{align*}
proving the first part of Theorem \ref{thm: convergence of hierarchical FL}.

Consequently, 
\begin{align*}
\norm{\frac{1}{T}\sum_{t=1}^T \pth{w_j[t] - \bar{z}[t]}}  
& = \norm{\frac{1}{T}\sum_{t=1}^{t_0-1} \pth{w_j[t] - \bar{z}[t]} + \frac{1}{T}\sum_{t=t_0}^{T} \pth{w_j[t] - \bar{z}[t]}} \\
& \le \frac{1}{T}\sum_{t=1}^{t_0-1} \norm{w_j[t] - \bar{z}[t]} + \frac{1}{T}\sum_{t=t_0}^{T} \norm{{w_j[t] - \bar{z}[t]}}\\
& \le \frac{1}{T}\frac{4M^2Lt_0^2}{\pth{\min_{i\in [M]}\beta_i}^{2D^*B}\norm{K}} + \frac{1}{T}\sum_{t=t_0}^{T}\frac{16M^2L}{\pth{\min_{i\in [M]}\beta_i}^{2D^*B}\norm{K}(1-b)t} \\
& \le \frac{1}{T}\frac{4M^2Lt_0^2}{\pth{\min_{i\in [M]}\beta_i}^{2D^*B}\norm{K}} + \frac{1}{T}\frac{16M^2L}{\pth{\min_{i\in [M]}\beta_i}^{2D^*B}\norm{K}(1-b)}\int_{t=t_0}^{T+1} \frac{1}{t} dt \\
& \le \frac{1}{T}\frac{4M^2Lt_0^2}{\pth{\min_{i\in [M]}\beta_i}^{2D^*B}\norm{K}} + \frac{16M^2L}{\pth{\min_{i\in [M]}\beta_i}^{2D^*B}\norm{K}(1-b)} \frac{1}{T}\log(T+1). 
\end{align*}

\paragraph{Bounding (a):}
\begin{align*}
\bar{z}[t] - w_t^*  
& = A\bar{z}[t-1] - \eta[t] \frac{1}{N}\sum_{j=1}^Ng_{j}[t] - w_{t}^* \\
& = A\bar{z}[t-1] - \eta[t] \frac{1}{N}\sum_{j=1}^N \pth{H_j^{\top}H_j\pth{\frac{z_j[t-1]}{m_j[t-1]} -w_{t-1}^*} + H_j^{\top}n_j[t-1]} - w_t^* \\
& =  A\pth{\bar{z}[t-1] - w_{t-1}^*} - \eta[t]\pth{\frac{1}{N}\sum_{j=1}^N H_j^{\top}H_j \pth{\frac{z_j[t-1]}{m_j[t-1]} -w_{t}^*}}\\
& \qquad - \eta[t] \frac{1}{N}\sum_{j=1}^N  H_j^{\top}n_j[t-1]\\
& =  A\pth{\bar{z}[t-1] - w_{t-1}^*} - \eta[t]\pth{\frac{1}{N}\sum_{j=1}^N H_j^{\top}H_j \pth{\bar{z}[t-1] - w_{t-1}^* +  \frac{z_j[t-1]}{m_j[t-1]} -\bar{z}[t-1]}}\\
& \qquad - \eta[t] \frac{1}{N}\sum_{j=1}^N  H_j^{\top}n_j[t-1]\\
& =  \pth{A - \eta[t] \frac{1}{N}\sum_{j=1}^N H_j^{\top}H_j}\pth{\bar{z}[t-1] - w_{t-1}^*}
- \eta[t] \frac{1}{N}\sum_{j=1}^N H_j^{\top}H_j\pth{\frac{z_j[t-1]}{m_j[t-1]} -\bar{z}[t-1]}\\
& \qquad - \eta[t] \frac{1}{N}\sum_{j=1}^N  H_j^{\top}n_j[t-1]\\
& = \pth{A - \frac{\eta[t]}{N}K}\pth{\bar{z}[t-1] - w_{t-1}^*}
- \eta[t] \frac{1}{N}\sum_{j=1}^N H_j^{\top}H_j\pth{\frac{z_j[t-1]}{m_j[t-1]} -\bar{z}[t-1]}\\
& \qquad - \eta[t] \frac{1}{N}\sum_{j=1}^N  H_j^{\top}n_j[t-1]. 
\end{align*}
For ease of exposition, let $C[t-1] = \eta[t] \frac{1}{N}\sum_{j=1}^N H_j^{\top} H_j\pth{\frac{z_j[t-1]}{m_j[t-1]} -\bar{z}[t-1]}$
and $W[t-1] =  \eta[t] \frac{1}{N}\sum_{j=1}^N  H_j^{\top}n_j[t-1]$. 
Notably, $\expect{W[t-1]} = \expect{\eta[t] \frac{1}{N}\sum_{j=1}^N  H_j^{\top}n_j[t-1]} = \bm{0}$. We unroll the dynamics of $\bar{z}[t] - w_t^* $ as
\begin{align*}
\bar{z}[t] - w_t^* & = \pth{A - \frac{\eta[t]}{N}K}\pth{\bar{z}[t-1] - w_{t-1}^*}
- C[t-1] - W[t-1] \\
& = \pth{A - \frac{\eta[t]}{N}K} \pth{A - \frac{\eta[t-1]}{N}K}\cdots \pth{A - \frac{\eta[1]}{N}K}\pth{\bar{z}[0] - w_{0}^*} \\
&\qquad - \sum_{r=2}^{t+1} \pth{A - \frac{\eta[t]}{N}K} \pth{A - \frac{\eta[t-1]}{N}K}\cdots \pth{A - \frac{\eta[r]}{N}K} \pth{C[r-2]+W[r-2]}. 
\end{align*}
Thus, 
\begin{align}
\label{eq: tracking centralized mimic}
\nonumber
\frac{1}{T}\sum_{t=1}^T\pth{\bar{z}[t] - w_t^*}    
& = \underbrace{\frac{1}{T}\sum_{t=1}^T \pth{A - \frac{\eta[t]}{N}K} \pth{A - \frac{\eta[t-1]}{N}K}\cdots \pth{A - \frac{\eta[1]}{N}K}\pth{\bar{z}[0] - w_{0}^*}}_{(A)} \\
\nonumber
& \qquad -  \underbrace{\frac{1}{T}\sum_{t=1}^T\sum_{r=2}^{t+1} \pth{A - \frac{\eta[t]}{N}K} \pth{A - \frac{\eta[t-1]}{N}K}\cdots \pth{A - \frac{\eta[r]}{N}K} C[r-2]}_{(B)}\\
& \qquad -  \underbrace{\frac{1}{T}\sum_{t=1}^T\sum_{r=2}^{t+1} \pth{A - \frac{\eta[t]}{N}K} \pth{A - \frac{\eta[t-1]}{N}K}\cdots \pth{A - \frac{\eta[r]}{N}K}W[r-2]}_{(C)}.  
\end{align}

Since $A$ is symmetric, it admits an eigenvalue decomposition, i.e., 
\[
A = U\Lambda U^{\top}, 
\]
where $U\in \reals^{d\times d}$ is the square $d\times d$ matrix whose $i$-th column is the $i$-th eigenvector of $A$, and $\Lambda$ is the diagonal matrix whose diagonal elements are the corresponding eigenvalues. 
Thus, 
\[
A - \eta[t]K = U\Lambda U^{\top} - \eta[t]K = U\pth{\Lambda - \eta[t] U^{\top}KU}U^{\top}. 
\]
For any $r$, it holds that 
\begin{align*}
& \pth{A - \frac{\eta[t]}{N}K} \pth{A - \frac{\eta[t-1]}{N}K}\cdots \pth{A - \frac{\eta[r]}{N}K}\\
& = U\pth{\Lambda - \eta[t] U^{\top}KU}U^{\top} U\pth{\Lambda - \eta[t-1] U^{\top}KU}U^{\top}\cdots 
U\pth{\Lambda - \eta[r] U^{\top}KU}U^{\top}\\
& = U\pth{\Lambda - \eta[t] U^{\top}KU}\pth{\Lambda - \eta[t-1] U^{\top}KU}\cdots 
\pth{\Lambda - \eta[r] U^{\top}KU}U^{\top}. 
\end{align*}
Thus, 
\begin{align*}
&\norm{\pth{A - \frac{\eta[t]}{N}K} \pth{A - \frac{\eta[t-1]}{N}K}\cdots \pth{A - \frac{\eta[r]}{N}K}}\\
&\le \norm{U\pth{\Lambda - \eta[t] U^{\top}KU}\pth{\Lambda - \eta[t-1] U^{\top}KU}\cdots 
\pth{\Lambda - \eta[r] U^{\top}KU}U^{\top}} \\
& = \norm{\pth{\Lambda - \eta[t] U^{\top}KU}\pth{\Lambda - \eta[t-1] U^{\top}KU}\cdots 
\pth{\Lambda - \eta[r] U^{\top}KU}} \\
& \le  \prod_{\tau=r}^t \norm{\Lambda - \eta[\tau] U^{\top}KU}. 
\end{align*}
Let $1\ge \lambda^d_1 \ge \cdots \ge \lambda_d^d\ge 0$ be the eigenvalues of the dynamic matrix $A$. 
Notably, $U$ is a rotation matrix. Thus, $U^{\top}KU$ and $K$ share the same set of eigenvalues. By definition, we have 
\begin{align*}
\norm{\Lambda - \eta[\tau] U^{\top}KU} & = \sup_{v\in \calS^d} v^{\top} \pth{\Lambda - \eta[\tau] U^{\top}KU} v\\
& = \sup_{v\in \calS^d} v^{\top} \Lambda v - \eta[\tau] \inf_{v\in \calS^d} v^{\top}U^{\top}KU v \\
& \le 1 - \eta[\tau] \lambda_d^o. 
\end{align*}
So, 
\begin{align*}
&\norm{\pth{A - \frac{\eta[t]}{N}K} \pth{A - \frac{\eta[t-1]}{N}K}\cdots \pth{A - \frac{\eta[r]}{N}K}} \\
&\le \prod_{\tau=r}^t \pth{1-\eta[\tau] \lambda_d^o} \\
& = \exp\pth{\ln \prod_{\tau=r}^t \pth{1-\eta[\tau] \lambda_d^o}} \\
& = \exp\pth{\sum_{\tau=r}^t \ln \pth{1-\eta[\tau] \lambda_d^o}}\\
& \le \exp\pth{\sum_{\tau=r}^t -\eta[\tau] \lambda_d^o} \\
& = \exp\pth{\frac{\lambda_1^o}{\lambda_d^o}} \exp\pth{-\sum_{\tau=r}^t \frac{1}{\tau}}\\
& \le \exp\pth{\frac{\lambda_1^o}{\lambda_d^o}} \exp\pth{ -\log (t) + \log (r-1)}\\
& = \exp\pth{\frac{\lambda_1^o}{\lambda_d^o}} \frac{r-1}{t}. 
\end{align*}

Besides, 
\begin{align*}
C[t-1] = \eta[t] \frac{1}{N}\sum_{j=1}^N H_j^{\top} H_j\pth{\frac{z_j[t-1]}{m_j[t-1]} -\bar{z}[t-1]}.  
\end{align*}

\paragraph{Bounding (A):}
\begin{align*}
&\norm{\frac{1}{T}\sum_{t=1}^T \pth{A - \frac{\eta[t]}{N}K} \pth{A - \frac{\eta[t-1]}{N}K}\cdots \pth{A - \frac{\eta[1]}{N}K}\pth{\bar{z}[0] - w_{0}^*}}\\
& \le \frac{1}{T}\sum_{t=1}^T\norm{\pth{A - \frac{\eta[t]}{N}K} \pth{A - \frac{\eta[t-1]}{N}K}\cdots \pth{A - \frac{\eta[1]}{N}K}} \norm{\bar{z}[0] - w_{0}^*}\\
& = \frac{1}{T}\sum_{t=1}^T\norm{\pth{A - \frac{\eta[t]}{N}K} \pth{A - \frac{\eta[t-1]}{N}K}\cdots \pth{A - \frac{\eta[1]}{N}K}} \norm{w_{0}^*}\\
& \le  \norm{w_{0}^*} \exp\pth{\frac{\lambda_1^o}{\lambda_d^o}}\frac{1}{T}\sum_{t=1}^T \frac{1}{t} \\
& \le \norm{w_{0}^*} \exp\pth{\frac{\lambda_1^o}{\lambda_d^o}}\frac{1}{T}\log (T+1).  
\end{align*}

\paragraph{Bounding (B):}
\begin{align*}
&\norm{\frac{1}{T}\sum_{t=1}^T\sum_{r=2}^{t+1} \pth{A - \frac{\eta[t]}{N}K} \pth{A - \frac{\eta[t-1]}{N}K}\cdots \pth{A - \frac{\eta[r]}{N}K} C[r-2]} \\
& \le \frac{1}{T}\sum_{t=1}^T\sum_{r=2}^{t+1} \norm{\pth{A - \frac{\eta[t]}{N}K} \pth{A - \frac{\eta[t-1]}{N}K}\cdots \pth{A - \frac{\eta[r]}{N}K}}\norm{C[r-2]} \\
& \le \exp\pth{\frac{\lambda_1^o}{\lambda_d^o}}\frac{1}{T}\sum_{t=1}^T\sum_{r=2}^{t+1} \frac{r-1}{t} \norm{\eta[r-1] \frac{1}{N}\sum_{j=1}^N H_j^{\top} H_j\pth{\frac{z_j[r-2]}{m_j[r-2]} -\bar{z}[r-2]}}\\
& \le \exp\pth{\frac{\lambda_1^o}{\lambda_d^o}}\frac{1}{T}\sum_{t=1}^T\sum_{r=2}^{t+1} \frac{r-1}{t}  \frac{1}{\norm{K} (r-1)}\frac{1}{N}\sum_{j=1}^N \norm{H_j^{\top} H_j}\norm{\pth{\frac{z_j[r-2]}{m_j[r-2]} -\bar{z}[r-2]}}\\
& \le \exp\pth{\frac{\lambda_1^o}{\lambda_d^o}}\frac{1}{T}\sum_{t=1}^T\sum_{r=2}^{t+1} \frac{1}{t} \max_{j}\norm{w_j[r-2]-\bar{z}[r-2]}\\
& = \exp\pth{\frac{\lambda_1^o}{\lambda_d^o}}\frac{1}{T} \sum_{t=0}^{T-1}\pth{\sum_{r=t+1}^T\frac{1}{r}}\max_{j}\norm{w_j[t]-\bar{z}[t]}. 
\end{align*}
Note that 
\begin{align*}
&\frac{1}{T}\exp\pth{\frac{\lambda_1^o}{\lambda_d^o}}\sum_{t=0}^{T-1}\pth{\sum_{r=t+1}^T\frac{1}{r}}\max_{j}\norm{w_j[t]-\bar{z}[t]}\\
& = \frac{1}{T}\exp\pth{\frac{\lambda_1^o}{\lambda_d^o}}\sum_{t=0}^{t_0-1} \pth{\sum_{r=t+1}^T\frac{1}{r}}\max_{j}\norm{w_j[t]-\bar{z}[t]}
+ \frac{1}{T}\exp\pth{\frac{\lambda_1^o}{\lambda_d^o}}\sum_{t=t_0}^{T-1}\pth{\sum_{r=t+1}^T\frac{1}{r}}\max_{j}\norm{w_j[t]-\bar{z}[t]}\\
& \le \frac{\exp\pth{\lambda_1^o/\lambda_d^o}4M^2Lt^2_0}{\pth{\min_{i\in [M]}\beta_i}^{2D^*B}\norm{K}}\frac{\log\pth{T+1}}{T} + \frac{16M^2L}{\pth{\min_{i\in [M]}\beta_i}^{2D^*B}\norm{K}(1-b)}\frac{\log^2(T+1)}{T}. 
\end{align*}

\paragraph{Bounding (C): Handling noises.}
We will use McDiarmid's inequality to derive high probability bound on term (C).   

We first observe that 
\begin{align*}
&\sum_{t=1}^T\sum_{r=2}^{t+1} \pth{A - \frac{\eta[t]}{N}K} \pth{A - \frac{\eta[t-1]}{N}K}\cdots \pth{A - \frac{\eta[r]}{N}K}W[r-2]  \\
& = \sum_{r=2}^{T-1}\sum_{t=r-1}^{T} \pth{A - \frac{\eta[t]}{N}K} \pth{A - \frac{\eta[t-1]}{N}K}\cdots \pth{A - \frac{\eta[r]}{N}K}W[r-2] 
\end{align*}
Note that the above quantity is a $d$-dimensional vector. We focus on each of the coordinate separately. 
Let's perturb the observation noise of agents at time $r^{\prime}-2$ and check its impacts on the $i$-th coordinate, where $i\in [d]$. 
It is easy to see that the difference on each of the coordinate is upper bounded by the $\ell_2$ norm of the corresponding quantities, which we can further bounded as follows: 
% \[
% \norm{\sum_{t=1}^T\sum_{r=2}^{t+1} \pth{A - \frac{\eta[t]}{N}K} \pth{A - \frac{\eta[t-1]}{N}K}\cdots \pth{A - \frac{\eta[r]}{N}K}W[r-2]}. 
% \]
\begin{align*}
\norm{\sum_{t=r^{\prime}-1}^{T} \pth{A - \frac{\eta[t]}{N}K} \pth{A - \frac{\eta[t-1]}{N}K}\cdots \pth{A - \frac{\eta[r^{\prime}]}{N}K}\pth{W[r^{\prime}-2] - \tilde{W}[r^{\prime}-2]}}
\le B_0\log T. 
\end{align*}
By McDiarmid's inequality, we obtain that with probability at most $\delta/d$, 
\begin{align*}
&\qth{\sum_{t=1}^T\sum_{r=2}^{t+1} \pth{A - \frac{\eta[t]}{N}K} \pth{A - \frac{\eta[t-1]}{N}K}\cdots \pth{A - \frac{\eta[r]}{N}K}W[r-2]}^i \\
&\qquad \qquad - \expect{\qth{\sum_{t=1}^T\sum_{r=2}^{t+1} \pth{A - \frac{\eta[t]}{N}K} \pth{A - \frac{\eta[t-1]}{N}K}\cdots \pth{A - \frac{\eta[r]}{N}K}W[r-2]}^i} \ge \sqrt{\frac{T}{2}\log d/\delta}\log T\\
& \Longleftrightarrow \\
&\qth{\sum_{t=1}^T\sum_{r=2}^{t+1} \pth{A - \frac{\eta[t]}{N}K} \pth{A - \frac{\eta[t-1]}{N}K}\cdots \pth{A - \frac{\eta[r]}{N}K}W[r-2]}^i \ge \sqrt{\frac{T}{2}\log (d/\delta)}B_0\log T. 
\end{align*}
By a union bound, we know that with probability at least $1-\delta$, 
\begin{align*}
\qth{\sum_{t=1}^T\sum_{r=2}^{t+1} \pth{A - \frac{\eta[t]}{N}K} \pth{A - \frac{\eta[t-1]}{N}K}\cdots \pth{A - \frac{\eta[r]}{N}K}W[r-2]}^i < \sqrt{\frac{T}{2}\log (d/\delta)}B_0\log T   ~~~ \forall ~ i=1, \cdots, d. 
\end{align*}
Therefore, we conclude that with probability at least $1-\delta$, 
\begin{align*}
\norm{\sum_{t=1}^T\sum_{r=2}^{t+1} \pth{A - \frac{\eta[t]}{N}K} \pth{A - \frac{\eta[t-1]}{N}K}\cdots \pth{A - \frac{\eta[r]}{N}K}W[r-2]} \le    \sqrt{\frac{dT}{2}\log (d/\delta)}B_0\log T. 
\end{align*}

Combining the bounds on terms  (A), (B), and (C), we bound Eq.\eqref{eq: tracking centralized mimic} as: With probability at least $1-\delta$, 
\begin{align*}
\frac{1}{T}\sum_{t=1}^T\pth{\bar{z}[t] - w_t^*} 
& \le  \norm{w_{0}^*} \exp\pth{\frac{\lambda_1^o}{\lambda_d^o}}\frac{1}{T}\log (T+1)
+ \frac{\exp\pth{\lambda_1^o/\lambda_d^o}4M^2Lt^2_0}{\pth{\min_{i\in [M]}\beta_i}^{2D^*B}\norm{K}}\frac{\log\pth{T+1}}{T} \\
& \qquad + \frac{16M^2L}{\pth{\min_{i\in [M]}\beta_i}^{2D^*B}\norm{K}(1-b)}\frac{\log^2(T+1)}{T} 
+ \sqrt{\frac{d}{2T}\log (d/\delta)}B_0\log T, 
\end{align*}
bounding term (a) in Eq.\,\eqref{eq: tracking average cumultive error}.

Therefore, we bound Eq.\,\eqref{eq: tracking average cumultive error} as 
\begin{align*}
\frac{1}{T}\sum_{t=1}^T \pth{w_j[t] - w_t^*}  
&\le \norm{w_{0}^*} \exp\pth{\frac{\lambda_1^o}{\lambda_d^o}}\frac{1}{T}\log (T+1)
+ \frac{\exp\pth{\lambda_1^o/\lambda_d^o}4M^2Lt^2_0}{\pth{\min_{i\in [M]}\beta_i}^{2D^*B}\norm{K}}\frac{\log\pth{T+1}}{T} \\
& \qquad + \frac{16M^2L}{\pth{\min_{i\in [M]}\beta_i}^{2D^*B}\norm{K}(1-b)}\frac{\log^2(T+1)}{T} 
+ \sqrt{\frac{d}{2T}\log (d/\delta)}\log T\\
& \qquad + \frac{1}{T}\frac{4M^2Lt_0^2}{\pth{\min_{i\in [M]}\beta_i}^{2D^*B}\norm{K}} + \frac{16M^2L}{\pth{\min_{i\in [M]}\beta_i}^{2D^*B}\norm{K}(1-b)} \frac{1}{T}\log(T+1)\\
& \le \norm{w_{0}^*} \exp\pth{\frac{\lambda_1^o}{\lambda_d^o}}\frac{\log (T+1)}{T}
+ \frac{\exp\pth{\lambda_1^o/\lambda_d^o}8M^2Lt^2_0}{\pth{\min_{i\in [M]}\beta_i}^{2D^*B}\norm{K}}\frac{\log\pth{T+1}}{T}\\
& \qquad + \frac{16M^2L}{\pth{\min_{i\in [M]}\beta_i}^{2D^*B}\norm{K}(1-b)}\frac{\log^2(T+1)}{T} 
+ \sqrt{\frac{d}{2T}\log (d/\delta)}B_0\log T. 
\end{align*}
\end{proof}
